# Supplementary material for: Analytic Representations of Bath Correlation Functions for Ohmic and Superohmic Spectral Densities Using Simple Poles
Source: arXiv:1405.2440 ancillary file (2014-08-19)
Supplement: Supplementary file 1 [file supporting_information.pdf]

# Analytic Representations of Bath Correlation Functions for Ohmic and Superohmic Spectral Densities Using Simple Poles

*Supporting Information*


Abstract

In this supporting information (SI) we provide the parameters for the fits to the spectral densities (SDs) we considered in the main text: the damped molecular vibration Eq. (17), the log-normal SD Eq. (18) and the sum of both. If nothing else is stated, all references given here are with respect to the main text.

We present the parameters for fits with different scaling parameters $n \in \{1, 3, 5\}$ of our fit functions Eq. (3), i.e. for different power-law scalings close to the frequency $\omega = 0$. Additionally, we present the resulting parameters for the corresponding bath correlation functions (BCF) at different temperatures $T \in \{4\text{ K}, 77\text{ K}, 300\text{ K}\}$. We show plots of all the fits that we provide here. For all considered temperatures we also show plots of the corresponding BCFs as well as the absorption spectra. We compare all the approximations given in this SI to the respective exact curves (BCFs and spectra) for each given SD.


## 1 Log-normal SD (Background)

The log-normal SD Eq. (18) has been suggested to describe the broad background of experimentally extracted SDs of bacteriochlorophyll molecules in pigment-protein complexes [29]. It shows a non-algebraic behavior for low frequencies as well as for high frequencies.

## 1.1 Fits for the log-normal SD

In Table I (SI) we provide the parameters for our fits to the log-normal SD from Ref. [29]. For $n = 3$ and $n = 5$ we take products with 3 poles $\omega_{j_k}$ for each summand in Eq. (3) into account in order to adjust the high-frequency behavior of our fit functions. For $n = 1$ we take 2 poles for every summand. For the cases $n = 3$ and $n = 5$ we use only one summand, whereas for $n = 1$ we use 4 summands (which amounts in total to 8 poles $\omega_{j_k}$ in the upper right part of the complex plane for $n = 1$) in order to enhance the agreement between the SD and our fit for smaller frequencies.

| | | $n = 1$ | $n = 3$ | $n = 5$ |
|---|---|---|---|---|
| $p_1$ | | 3.6981e+09 | 1.7661e+10 | 2.4229e5 |
| | $\omega_{1_1}$ | 125.69+65.995j | 14.709+29.995j | 5.5219+11.255j |
| | $\omega_{1_2}$ | 297.83+222.87j | 41.127+91.783j | 15.443+34.436j |
| | $\omega_{1_3}$ | | 137.60+272.05j | 51.693+102.07j |
| | | | | |
| $p_2$ | | 3.4283e+05 | | |
| | $\omega_{2_1}$ | 24.177+6.8901j | | |
| | $\omega_{2_2}$ | 61.146+7.7632j | | |
| | | | | |
| $p_3$ | | 5.9692e+05 | | |
| | $\omega_{3_1}$ | 33.176+10.937j | | |
| | $\omega_{3_2}$ | 52.446+11.077j | | |
| | | | | |
| $p_4$ | | 3.2796e+07 | | |
| | $\omega_{4_1}$ | 112.26+36.733j | | |
| | $\omega_{4_2}$ | 65.201+22.859j | | |
| | | | | |

Table I (SI): Fit parameters for the log-normal SD according to Eqs. (3), (4) for three different scaling parameters $n \in \{1, 3, 5\}$.

## 1.2 Resulting parameters for the BCFs corresponding to our fits of the log-normal SD

Here, we provide the coefficients of the exponential decomposition Eq. (2) of the BCF for the different fits of the log-normal SD from Table I (SI) and different temperatures $T \in \{4\ \text{K}, 77\ \text{K}, 300\ \text{K}\}$.

### 1.2.1 Parameters for the BCFs corresponding to the fit of the log-normal SD for n=1

In Table II (SI) we list the parameters of the exponential decompositions Eq. (2) of the BCFs (according to Eq. (6)) for the scaling parameter $n = 1$, i.e. an ohmic fit function with a linear behavior at frequency zero. For $T = 4$ K we take 11 Padé expansion terms for the hyperbolic cotangent into account, for $T = 77$ K we take 2 terms and for $T = 300$ K we take 1 term.

### 1.2.2 Parameters for the BCF corresponding to the fit for n=3

In Table III (SI) we list the parameters of the exponential decomposition Eq. (2) of the BCF (according to Eq. (6)) for the scaling parameter $n = 3$, i.e. a superohmic fit function with a cubic behavior at frequency zero. For $T = 4$ K we take 14 Padé expansion terms for the hyperbolic cotangent into account, for $T = 77$ K we take 2 terms and for $T = 300$ K we take 1 term.

### 1.2.3 Parameters for the BCF corresponding to the fit for n=5

In Table IV (SI) we list the parameters of the exponential decomposition Eq. (2) of the BCF (according to Eq. (6)) for the scaling parameter $n = 5$, i.e. a superohmic fit function with a behavior proportional to $\omega^5$ at frequency zero. For $T = 4$ K we take 15 Padé expansion terms for the hyperbolic cotangent into account, for $T = 77$ K we take 3 terms and for $T = 300$ K we take 1 term.

| $T = 4$ K | $p_m$ | $\omega_m$ |
|---|---|---|
| | -4.7371e-18+1.5626e-17j | 1.2569e+02+6.5995e+01j |
| | 6.1816e-45-1.2636e-45j | 2.9783e+02+2.2287e+02j |
| | -2.9753e-03-4.8109e-03j | 2.4177e+01+6.8901e+00j |
| | -8.4164e-09+4.3624e-10j | 6.1146e+01+7.7632e+00j |
| | -6.3505e-04-3.3146e-05j | 3.3176e+01+1.0937e+01j |
| | 8.0172e-08+6.0801e-07j | 5.2446e+01+1.1077e+01j |
| | -3.8931e-16-1.5628e-16j | 1.1226e+02+3.6733e+01j |
| | 6.1569e-09-2.4373e-08j | 6.5201e+01+2.2859e+01j |
| | 6.8473e+02-2.0758e+02j | -1.2569e+02+6.5995e+01j |
| | -4.2431e+01+2.0758e+02j | -2.9783e+02+2.2287e+02j |
| | 3.1737e+01-1.1716e+01j | -2.4177e+01+6.8901e+00j |
| | 2.7648e+01+1.1721e+01j | -6.1146e+01+7.7632e+00j |
| | 6.4290e+01-7.2376e+01j | -3.3176e+01+1.0937e+01j |
| | 6.2428e+01+7.2376e+01j | -5.2446e+01+1.1077e+01j |
| | 8.9275e+01+2.2240e+02j | -1.1226e+02+3.6733e+01j |
| | 3.1439e+02-2.2240e+02j | -6.5201e+01+2.2859e+01j |
| | -1.0149e+01-1.2346e-15j | 0.0000e+00+1.7468e+01j |
| | -1.2419e+01+1.2346e-15j | 0.0000e+00+3.4936e+01j |
| | -1.2900e+01-1.2346e-15j | 0.0000e+00+5.2404e+01j |
| | -1.2465e+01+0.0000e+00j | 0.0000e+00+6.9873e+01j |
| | -1.1437e+01+4.6301e-16j | 0.0000e+00+8.7341e+01j |
| | -1.0038e+01+0.0000e+00j | 0.0000e+00+1.0484e+02j |
| | -9.6819e+00-3.7259e-16j | 0.0000e+00+1.2360e+02j |
| | -1.0632e+01+0.0000e+00j | 0.0000e+00+1.5087e+02j |
| | -5.1162e+00+1.3207e-15j | 0.0000e+00+2.0302e+02j |
| | 1.3255e+01+9.4554e-16j | 0.0000e+00+3.3007e+02j |
| | 3.6364e+00+2.6933e-16j | 0.0000e+00+9.7842e+02j |
| $T = 77$ K | $p_m$ | $\omega_m$ |
| | 3.6076e+01-6.0291e+01j | 1.2569e+02+6.5995e+01j |
| | 7.6069e-01+2.7730e-01j | 2.9783e+02+2.2287e+02j |
| | 5.7018e+01+3.9485e-01j | 2.4177e+01+6.8901e+00j |
| | 1.1421e+01-8.0391e+00j | 6.1146e+01+7.7632e+00j |
| | 9.8212e+01+4.3080e+01j | 3.3176e+01+1.0937e+01j |
| | 2.1056e+01-5.2196e+01j | 5.2446e+01+1.1077e+01j |
| | -1.2323e+01-2.9946e+01j | 1.1226e+02+3.6733e+01j |
| | 1.5365e+02+3.4506e+00j | 6.5201e+01+2.2859e+01j |
| | 7.2081e+02-1.4729e+02j | -1.2569e+02+6.5995e+01j |
| | -4.1670e+01+2.0730e+02j | -2.9783e+02+2.2287e+02j |
| | 8.8758e+01-1.2116e+01j | -2.4177e+01+6.8901e+00j |
| | 3.9069e+01+1.9760e+01j | -6.1146e+01+7.7632e+00j |
| | 1.6250e+02-1.1546e+02j | -3.3176e+01+1.0937e+01j |
| | 8.3484e+01+1.2457e+02j | -5.2446e+01+1.1077e+01j |
| | 7.6952e+01+2.5234e+02j | -1.1226e+02+3.6733e+01j |
| | 4.6804e+02-2.2585e+02j | -6.5201e+01+2.2859e+01j |
| | 2.1343e+01+0.0000e+00j | 0.0000e+00+3.3748e+02j |
| | 2.7740e+00+0.0000e+00j | 0.0000e+00+1.0436e+03j |
| $T = 300$ K | $p_m$ | $\omega_m$ |
| | 7.1876e+02-2.7319e+02j | 1.2569e+02+6.5995e+01j |
| | -5.5725e+01-3.7440e+00j | 2.9783e+02+2.2287e+02j |
| | 2.6423e+02+1.5684e+01j | 2.4177e+01+6.8901e+00j |
| | 7.4677e+01-4.5456e+01j | 6.1146e+01+7.7632e+00j |
| | 4.6811e+02+2.5520e+02j | 3.3176e+01+1.0937e+01j |
| | 1.4983e+02-2.9070e+02j | 5.2446e+01+1.1077e+01j |
| | -9.7366e+00-3.1959e+02j | 1.1226e+02+3.6733e+01j |
| | 9.6639e+02+2.1691e+02j | 6.5201e+01+2.2859e+01j |
| | 1.4035e+03+6.5615e+01j | -1.2569e+02+6.5995e+01j |
| | -9.8156e+01+2.1132e+02j | -2.9783e+02+2.2287e+02j |
| | 2.9597e+02-2.7405e+01j | -2.4177e+01+6.8901e+00j |
| | 1.0232e+02+5.7177e+01j | -6.1146e+01+7.7632e+00j |
| | 5.3240e+02-3.2757e+02j | -3.3176e+01+1.0937e+01j |
| | 2.1226e+02+3.6307e+02j | -5.2446e+01+1.1077e+01j |
| | 7.9539e+01+5.4199e+02j | -1.1226e+02+3.6733e+01j |
| | 1.2808e+03-4.3931e+02j | -6.5201e+01+2.2859e+01j |

| | | |
|---|---|---|
| | 5.6054e-01+0.0000e+00j | 0.0000e+00+1.6151e+03j |

Table II (SI): Parameters for the BCF decomposition Eq. (2) for our fit of the log-normal SD with $n = 1$ for 3 different temperatures $T \in \{4\ \mathrm{K}, 77\ \mathrm{K}, 300\ \mathrm{K}\}$.

| $T = 4$ K | $p_m$ | $\omega_m$ |
|---|---|---|
| | -1.8461e+00-4.0609e+00j | 1.4709e+01+2.9995e+01j |
| | -2.2573e-05-1.1358e-03j | 4.1127e+01+9.1783e+01j |
| | 7.9254e-20-9.9991e-20j | 1.3760e+02+2.7205e+02j |
| | -7.1391e+02-5.2398e+02j | -1.4709e+01+2.9995e+01j |
| | 3.0202e+03-2.2080e+01j | -4.1127e+01+9.1783e+01j |
| | -6.9406e+02+5.5012e+02j | -1.3760e+02+2.7205e+02j |
| | 4.6855e+01+8.8296e-15j | 0.0000e+00+1.7468e+01j |
| | 2.3380e+02-2.3546e-14j | 0.0000e+00+3.4936e+01j |
| | 2.1471e+01+0.0000e+00j | 0.0000e+00+5.2404e+01j |
| | -1.6603e+02-2.3546e-14j | 0.0000e+00+6.9873e+01j |
| | -2.8805e+02+0.0000e+00j | 0.0000e+00+8.7341e+01j |
| | -2.7459e+02+0.0000e+00j | 0.0000e+00+1.0481e+02j |
| | -1.7873e+02+2.7048e-14j | 0.0000e+00+1.2228e+02j |
| | -9.7641e+01-1.2008e-14j | 0.0000e+00+1.3983e+02j |
| | -4.9972e+01+0.0000e+00j | 0.0000e+00+1.5899e+02j |
| | -2.5355e-01+0.0000e+00j | 0.0000e+00+1.8591e+02j |
| | 8.6326e+01+1.3619e-14j | 0.0000e+00+2.3089e+02j |
| | 1.6000e+02-3.2185e-15j | 0.0000e+00+3.1547e+02j |
| | 5.0929e+01+3.0632e-15j | 0.0000e+00+5.1766e+02j |
| | 1.5955e+00+0.0000e+00j | 0.0000e+00+1.5413e+03j |
| $T = 77$ K | $p_m$ | $\omega_m$ |
| | 5.7203e+02+1.1116e+03j | 1.4709e+01+2.9995e+01j |
| | -6.2342e+02-1.0325e+03j | 4.1127e+01+9.1783e+01j |
| | 2.5263e+01-6.4693e+01j | 1.3760e+02+2.7205e+02j |
| | -1.4004e+02-1.6396e+03j | -1.4709e+01+2.9995e+01j |
| | 2.3968e+03+1.0105e+03j | -4.1127e+01+9.1783e+01j |
| | -6.6879e+02+6.1481e+02j | -1.3760e+02+2.7205e+02j |
| | 3.8096e+02+3.1994e-14j | 0.0000e+00+3.3748e+02j |
| | 7.6174e+00+3.4522e-15j | 0.0000e+00+1.0436e+03j |
| $T = 300$ K | $p_m$ | $\omega_m$ |
| | 1.3477e+03+5.1719e+03j | 1.4709e+01+2.9995e+01j |
| | 1.1413e+03-5.5949e+03j | 4.1127e+01+9.1783e+01j |
| | -1.8408e+02+4.2029e+02j | 1.3760e+02+2.7205e+02j |
| | 6.3567e+02-5.7000e+03j | -1.4709e+01+2.9995e+01j |
| | 4.1615e+03+5.5728e+03j | -4.1127e+01+9.1783e+01j |
| | -8.7814e+02+1.2983e+02j | -1.3760e+02+2.7205e+02j |
| | 1.3398e+00-1.1248e-15j | 0.0000e+00+1.6151e+03j |

Table III (SI): Parameters for the BCF decomposition Eq. (2) for our fit of the log-normal SD with $n = 3$ for 3 different temperatures $T \in \{4\ \mathrm{K}, 77\ \mathrm{K}, 300\ \mathrm{K}\}$.

| $T = 4$ K | $p_m$ | $\omega_m$ |
|---|---|---|
| | 3.2261e+00+3.2153e+00j | 5.5219e+00+1.1255e+01j |
| | -3.4409e+00+2.6437e+00j | 1.5443e+01+3.4436e+01j |
| | 1.9050e-05+1.6683e-05j | 5.1693e+01+1.0207e+02j |
| | 3.9637e+00+3.2956e+01j | -5.5219e+00+1.1255e+01j |
| | -7.5276e+02-8.3121e+02j | -1.5443e+01+3.4436e+01j |
| | 2.9044e+03+7.9239e+02j | -5.1693e+01+1.0207e+02j |
| | -2.0658e+01-7.0162e-15j | 0.0000e+00+1.7468e+01j |
| | 2.5302e+02+7.0162e-15j | 0.0000e+00+3.4936e+01j |
| | 1.8325e+02+5.3279e-14j | 0.0000e+00+5.2404e+01j |
| | -5.6323e-01+0.0000e+00j | 0.0000e+00+6.9873e+01j |
| | -1.3676e+02+3.4259e-14j | 0.0000e+00+8.7341e+01j |
| | -2.1734e+02+1.7760e-14j | 0.0000e+00+1.0481e+02j |
| | -2.2062e+02-1.6451e-14j | 0.0000e+00+1.2228e+02j |
| | -1.7892e+02-5.2728e-15j | 0.0000e+00+1.3975e+02j |
| | -1.3929e+02+9.0009e-15j | 0.0000e+00+1.5754e+02j |
| | -1.2717e+02+6.5987e-15j | 0.0000e+00+1.7851e+02j |
| | -1.1979e+02+1.0002e-14j | 0.0000e+00+2.0970e+02j |
| | -1.0013e+02-2.1017e-14j | 0.0000e+00+2.6165e+02j |
| | -7.3061e+01+1.8681e-14j | 0.0000e+00+3.5862e+02j |
| | -4.3831e+01+1.2033e-14j | 0.0000e+00+5.8964e+02j |
| | -1.4552e+01-1.6799e-14j | 0.0000e+00+1.7572e+03j |
| $T = 77$ K | $p_m$ | $\omega_m$ |
| | -1.3697e+02-5.3053e+01j | 5.5219e+00+1.1255e+01j |
| | 9.4904e+02+1.0160e+03j | 1.5443e+01+3.4436e+01j |
| | -7.6670e+02-5.9391e+02j | 5.1693e+01+1.0207e+02j |
| | -1.3623e+02+8.9224e+01j | -5.5219e+00+1.1255e+01j |
| | 1.9972e+02-1.8446e+03j | -1.5443e+01+3.4436e+01j |
| | 2.1377e+03+1.3863e+03j | -5.1693e+01+1.0207e+02j |
| | -2.1970e+02+0.0000e+00j | 0.0000e+00+3.3627e+02j |
| | -3.0150e+01-1.3008e-14j | 0.0000e+00+6.9350e+02j |
| | -1.1724e+01+1.3202e-14j | 0.0000e+00+1.9330e+03j |
| $T = 300$ K | $p_m$ | $\omega_m$ |
| | -5.3491e+02-2.5799e+02j | 5.5219e+00+1.1255e+01j |
| | 2.8416e+03+5.2311e+03j | 1.5443e+01+3.4436e+01j |
| | -2.5598e+02-4.8763e+03j | 5.1693e+01+1.0207e+02j |
| | -5.3417e+02+2.9416e+02j | -5.5219e+00+1.1255e+01j |
| | 2.0923e+03-6.0596e+03j | -1.5443e+01+3.4436e+01j |
| | 2.6484e+03+5.6687e+03j | -5.1693e+01+1.0207e+02j |
| | -1.7507e+01-2.2386e-14j | 0.0000e+00+1.6151e+03j |

Table IV (SI): Parameters for the BCF decomposition Eq. (2) for our fit of the log-normal SD with $n = 5$ for 3 different temperatures $T \in \{4\ \mathrm{K}, 77\ \mathrm{K}, 300\ \mathrm{K}\}$.

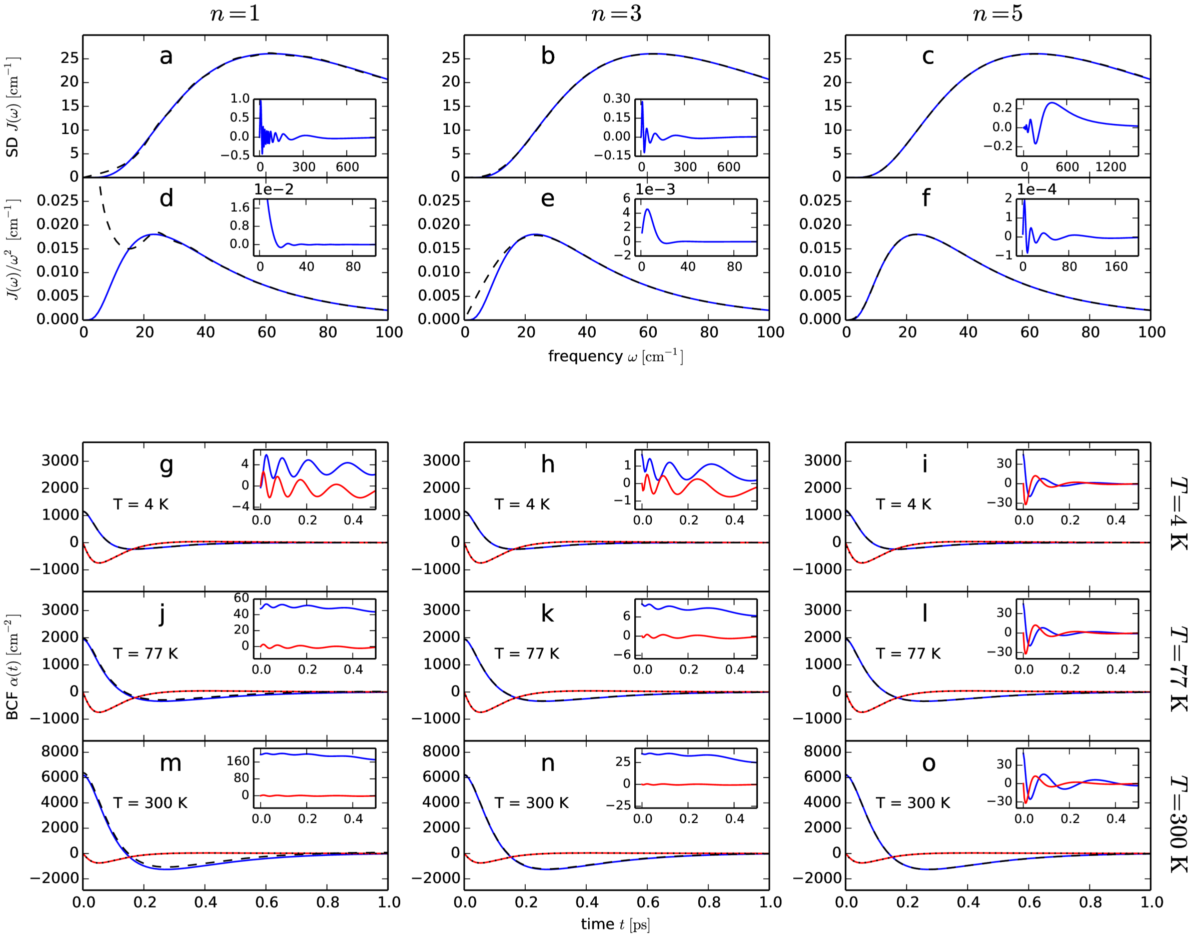


Figure 1 (SI): Log-normal SD, Eq. (18) and fits for different $n$; left column $n = 1$, middle column $n = 3$ and right column $n = 5$: The first row shows the SD (blue solid line) together with a fit according to the parameters given in Table I of the SI (black, dashed). The insets show the difference between the original SD and the approximations. Second row: SD divided by $\omega^2$. Rows three to five: Corresponding BCFs for three temperatures using the Padé approximation of the hyperbolic cotangent. Blue and red correspond to the exact real and imaginary parts, respectively. The gray dashed/dotted curves are the approximations based on the Tables II, III, IV of the SI. In the insets the differences are shown.

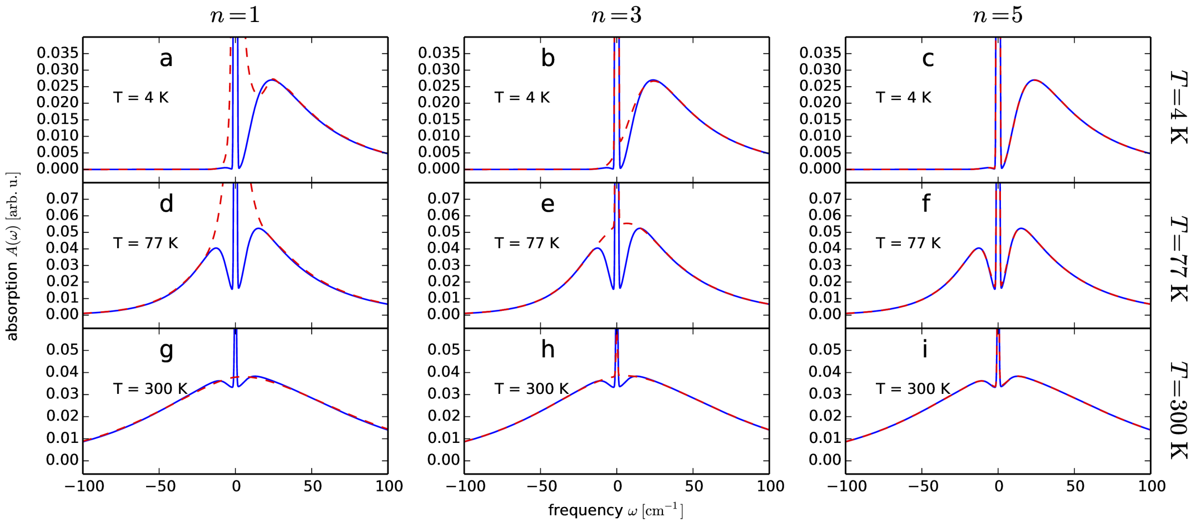


Figure 2 (SI): Absorption spectra for the log-normal SD according to Eq. (18), which is shown in Fig. 3 (b). The solid blue curve is the exact spectrum and the dashed red curve the one obtained from our fit. In the left column (panels (a), (d), (g)) the fit was performed with $n = 1$, in the middle column (panels (b), (e), (h)) with $n = 3$ and in the right column (panels (c), (f), (i)) with $n = 5$. The parameters for the respective fits are given in Tables II, III, IV of the SI. The first row is for $T = 4$ K, the second for 77 K and the third for 300 K.

# 2 Damped Vibrational Mode

We consider an SD of a vibrational mode related to shifted harmonic potential surfaces that is coupled to an ohmic bath with exponential cutoff. This model is discussed e.g. in Ref. [37]. This SD Eq. (17) has a cubic behavior at small $\omega$ and falls off like $e^{-\omega}/\omega$ for large $\omega$.

## 2.1 Fits for the SD of the damped vibrational mode

In Table V (SI) we provide the parameters for our fits to the SD of the damped vibrational mode from Ref. [37]. For all considered scaling parameters $n \in \{1, 3, 5\}$ we approximate this SD by one summand in Eq. (3). For $n = 5$ we take a product with 3 poles $\omega_{j_k}$ into account in order to adjust the high-frequency behavior of our fit functions. For $n = 1$ and $n = 3$ we take 2 poles.

| | | $n = 1$ | $n = 3$ | $n = 5$ |
|---|---|---|---|---|
| $p_1$ | | 2.4339e+08 | 9.6501e+03 | 1.2700e+04 |
| | $\omega_{1_1}$ | 183.02+9.1263j | 183.05+9.1885j | 183.05+9.1738j |
| | $\omega_{1_2}$ | 261.23+139.66j | 95.468+161.08j | 67.569+178.12j |
| | $\omega_{1_3}$ | | | 1.7613+11.123j |

Table V (SI): Fit parameters for the SD of the damped vibrational mode according to Eqs. (3), (4) for three different scaling parameters $n \in \{1, 3, 5\}$.

## 2.2 Resulting parameters for the BCFs corresponding to our fits of the SD of the damped vibrational mode

Here, we provide the coefficients of the exponential decomposition Eq. (2) of the BCF for the different fits of the SD of the damped vibrational mode from Table V (SI) for different temperatures $T \in \{4\text{ K}, 77\text{ K}, 300\text{ K}\}$.

### 2.2.1 Parameters for the BCF corresponding to the fit for n=1

In Table VI (SI) we list the parameters of the exponential decomposition Eq. (2) of the BCF (according to Eq. (6)) for the scaling parameter $n = 1$, i.e. an ohmic fit function with a linear behavior at frequency zero. For $T = 4$ K we take 8 Padé expansion terms for the hyperbolic cotangent into account, for $T = 77$ K we take 1 term and for $T = 300$ K we take 1 term.

| $T = 4$ K | $p_m$ | $\omega_m$ |
|---|---|---|
| | -2.1023e-28+3.7609e-27j<br>2.9190e-41-1.7778e-41j<br>1.0411e+03-5.8197e+01j<br>-3.5444e+01+5.8197e+01j<br>-2.6317e-01-7.7164e-17j<br>-4.8523e-01+7.7164e-17j<br>-6.3698e-01+0.0000e+00j<br>-7.0965e-01+7.7395e-17j<br>-8.1909e-01-2.2525e-17j<br>-1.3265e+00-4.3919e-17j<br>-1.1568e+00+0.0000e+00j<br>1.4512e+00-1.0253e-16j | 1.8302e+02+9.1263e+00j<br>2.6123e+02+1.3966e+02j<br>-1.8302e+02+9.1263e+00j<br>-2.6123e+02+1.3966e+02j<br>0.0000e+00+1.7468e+01j<br>0.0000e+00+3.4936e+01j<br>0.0000e+00+5.2404e+01j<br>0.0000e+00+6.9881e+01j<br>0.0000e+00+8.8211e+01j<br>0.0000e+00+1.1612e+02j<br>0.0000e+00+1.8496e+02j<br>0.0000e+00+5.4302e+02j |
| $T = 77$ K | $p_m$ | $\omega_m$ |
| | 3.4997e+01-4.2350e+00j<br>9.6513e-03+5.1361e-01j<br>1.0761e+03-5.3962e+01j<br>-3.5434e+01+5.7683e+01j<br>2.4454e+00+2.3210e-16j | 1.8302e+02+9.1263e+00j<br>2.6123e+02+1.3966e+02j<br>-1.8302e+02+9.1263e+00j<br>-2.6123e+02+1.3966e+02j<br>0.0000e+00+4.1455e+02j |
| $T = 300$ K | $p_m$ | $\omega_m$ |
| | 7.4090e+02-1.4099e+01j<br>-2.4251e+01-3.1531e+00j<br>1.7820e+03-4.4097e+01j<br>-5.9695e+01+6.1350e+01j<br>3.7688e-02+0.0000e+00j | 1.8302e+02+9.1263e+00j<br>2.6123e+02+1.3966e+02j<br>-1.8302e+02+9.1263e+00j<br>-2.6123e+02+1.3966e+02j<br>0.0000e+00+1.6151e+03j |

Table VI (SI): Parameters for the BCF decomposition Eq. (2) for our fit of the SD of the damped vibrational mode with $n = 1$ for 3 different temperatures $T \in \{4\ \mathrm{K}, 77\ \mathrm{K}, 300\ \mathrm{K}\}$.

### 2.2.2 Parameters for the BCF corresponding to the fit for n=3

In Table VII (SI) we list the parameters of the exponential decomposition Eq. (2) of the BCF (according to Eq. (6)) for the scaling parameter $n = 3$, i.e. a superohmic fit function with a cubic behavior at frequency zero. For $T = 4$ K we take 10 Padé expansion terms for the hyperbolic cotangent into account, for $T = 77$ K we take 2 terms and for $T = 300$ K we take 1 term.

| $T = 4$ K | $p_m$ | $\omega_m$ |
|---|---|---|
| | -2.2775e-28+4.3464e-27j | 1.8305e+02+9.1885e+00j |
| | -7.5986e-14+1.7536e-14j | 9.5468e+01+1.6108e+02j |
| | 1.0494e+03-5.4989e+01j | -1.8305e+02+9.1885e+00j |
| | -2.9849e+01+5.4989e+01j | -9.5468e+01+1.6108e+02j |
| | 7.7924e-03+2.8742e-18j | 0.0000e+00+1.7468e+01j |
| | 5.8962e-02+0.0000e+00j | 0.0000e+00+3.4936e+01j |
| | 1.8124e-01+3.8802e-17j | 0.0000e+00+5.2404e+01j |
| | 3.7592e-01+3.4491e-17j | 0.0000e+00+6.9873e+01j |
| | 6.1427e-01+7.1956e-17j | 0.0000e+00+8.7345e+01j |
| | 9.0685e-01-1.4090e-17j | 0.0000e+00+1.0521e+02j |
| | 1.6351e+00+0.0000e+00j | 0.0000e+00+1.2822e+02j |
| | 1.2812e+00-4.8943e-16j | 0.0000e+00+1.7122e+02j |
| | -9.9515e+00+0.0000e+00j | 0.0000e+00+2.7698e+02j |
| | -9.1832e+00-1.1536e-15j | 0.0000e+00+8.1913e+02j |
| $T = 77$ K | $p_m$ | $\omega_m$ |
| | 3.5231e+01-4.4310e+00j | 1.8305e+02+9.1885e+00j |
| | 3.3791e+00+8.3508e+00j | 9.5468e+01+1.6108e+02j |
| | 1.0846e+03-5.0558e+01j | -1.8305e+02+9.1885e+00j |
| | -2.6470e+01+4.6638e+01j | -9.5468e+01+1.6108e+02j |
| | -1.6101e+01-4.9991e-16j | 0.0000e+00+3.3748e+02j |
| | -5.6765e+00+0.0000e+00j | 0.0000e+00+1.0436e+03j |
| $T = 300$ K | $p_m$ | $\omega_m$ |
| | 7.4643e+02-1.7186e+01j | 1.8305e+02+9.1885e+00j |
| | -5.2331e+01+2.0795e+01j | 9.5468e+01+1.6108e+02j |
| | 1.7958e+03-3.7802e+01j | -1.8305e+02+9.1885e+00j |
| | -8.2180e+01+3.4194e+01j | -9.5468e+01+1.6108e+02j |
| | -2.5920e+00-5.6240e-16j | 0.0000e+00+1.6151e+03j |

Table VII (SI): Parameters for the BCF decomposition Eq. (2) for our fit of the SD of the damped vibrational mode with $n = 3$ for 3 different temperatures $T \in \{4\text{ K}, 77\text{ K}, 300\text{ K}\}$.

### 2.2.3 Parameters for the BCF corresponding to the fit for n=5

In Table VIII (SI) we list the parameters of the exponential decomposition Eq. (2) of the BCF (according to Eq. (6)) for the scaling parameter $n = 5$, i.e. a superohmic fit function with a behavior proportional to $\omega^5$ at frequency zero. For $T = 4$ K we take 11 Padé expansion terms for the hyperbolic cotangent into account, for $T = 77$ K we take 2 terms and for $T = 300$ K we take 1 term.

| $T = 4$ K | $p_m$ | $\omega_m$ |
|---|---|---|
| | -2.2071e-28+4.2011e-27j | 1.8305e+02+9.1738e+00j |
| | -1.6149e-09-1.9259e-11j | 6.7569e+01+1.7812e+02j |
| | -2.9801e-03+5.0132e-03j | 1.7613e+00+1.1123e+01j |
| | 1.0475e+03-5.5031e+01j | -1.8305e+02+9.1738e+00j |
| | -1.8328e+01+5.5024e+01j | -6.7569e+01+1.7812e+02j |
| | 1.0821e-02+1.9142e-03j | -1.7613e+00+1.1123e+01j |
| | -4.3867e-03+0.0000e+00j | 0.0000e+00+1.7468e+01j |
| | 6.0163e-02-1.3704e-17j | 0.0000e+00+3.4936e+01j |
| | 2.0837e-01+0.0000e+00j | 0.0000e+00+5.2404e+01j |
| | 4.6183e-01-5.4814e-17j | 0.0000e+00+6.9873e+01j |
| | 8.1051e-01-3.3458e-17j | 0.0000e+00+8.7341e+01j |
| | 1.2248e+00+6.5734e-17j | 0.0000e+00+1.0484e+02j |
| | 1.9369e+00-1.2148e-16j | 0.0000e+00+1.2360e+02j |
| | 3.4754e+00+0.0000e+00j | 0.0000e+00+1.5087e+02j |
| | -3.1129e+00-1.0448e-15j | 0.0000e+00+2.0302e+02j |
| | -1.5548e+01+3.6745e-16j | 0.0000e+00+3.3007e+02j |
| | -8.0855e+00+0.0000e+00j | 0.0000e+00+9.7842e+02j |
| $T = 77$ K | $p_m$ | $\omega_m$ |
| | 3.5171e+01-4.4084e+00j | 1.8305e+02+9.1738e+00j |
| | 5.7771e+00+1.1454e+01j | 6.7569e+01+1.7812e+02j |
| | -2.9000e-02-6.6243e-02j | 1.7613e+00+1.1123e+01j |
| | 1.0827e+03-5.0622e+01j | -1.8305e+02+9.1738e+00j |
| | -1.2550e+01+4.3570e+01j | -6.7569e+01+1.7812e+02j |
| | -1.5199e-02+7.3170e-02j | -1.7613e+00+1.1123e+01j |
| | -2.4124e+01+1.5203e-15j | 0.0000e+00+3.3748e+02j |
| | -6.8944e+00-2.3903e-15j | 0.0000e+00+1.0436e+03j |
| $T = 300$ K | $p_m$ | $\omega_m$ |
| | 7.4510e+02-1.6966e+01j | 1.8305e+02+9.1738e+00j |
| | -5.0828e+01+2.2055e+01j | 6.7569e+01+1.7812e+02j |
| | -9.3577e-02-2.6892e-01j | 1.7613e+00+1.1123e+01j |
| | 1.7926e+03-3.8065e+01j | -1.8305e+02+9.1738e+00j |
| | -6.9156e+01+3.2969e+01j | -6.7569e+01+1.7812e+02j |
| | -7.9776e-02+2.7585e-01j | -1.7613e+00+1.1123e+01j |
| | -3.1144e+00-6.9955e-16j | 0.0000e+00+1.6151e+03j |

Table VIII (SI): Parameters for the BCF decomposition Eq. (2) for our fit of the SD of the damped vibrational mode with $n = 5$ for 3 different temperatures $T \in \{4\ \mathrm{K}, 77\ \mathrm{K}, 300\ \mathrm{K}\}$.

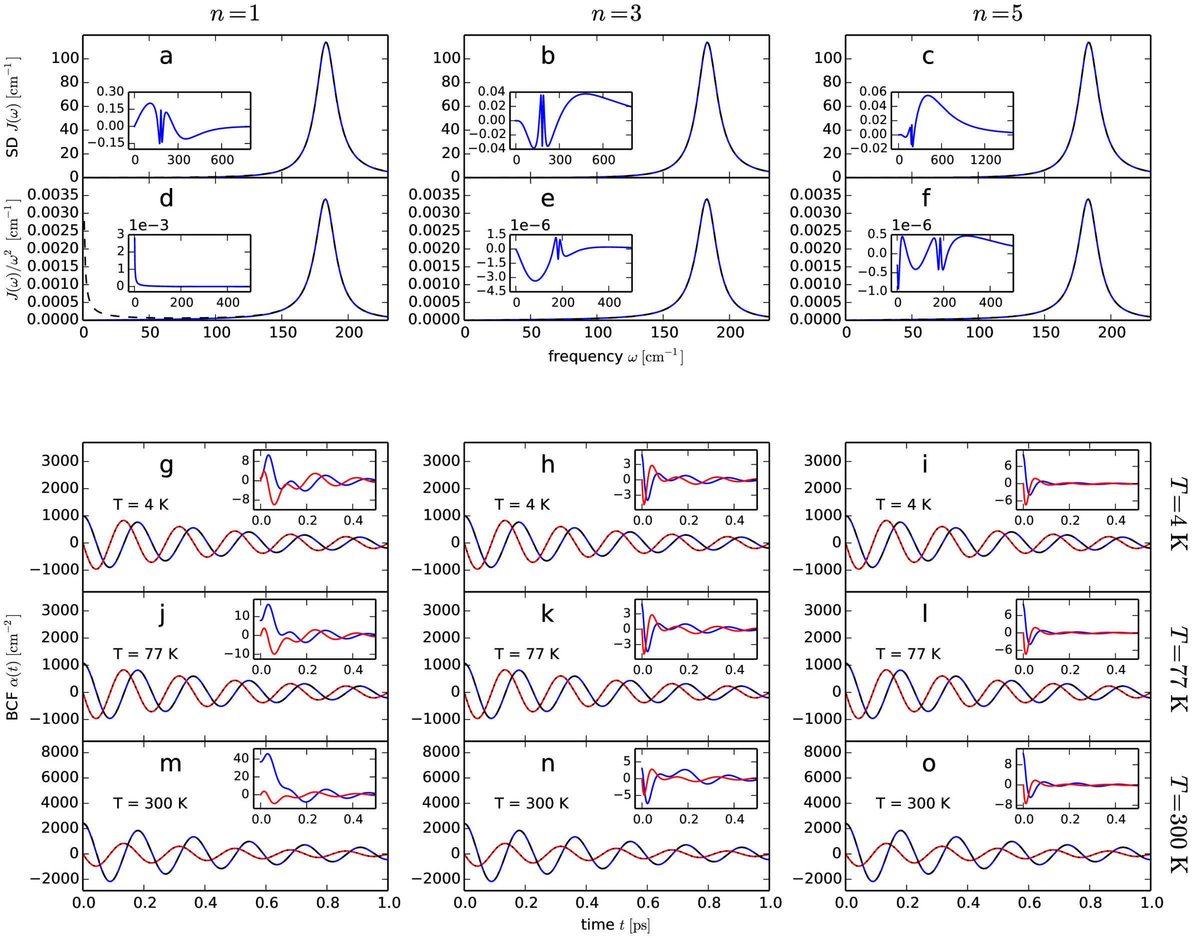


Figure 3 (SI): SD of the damped vibrational mode, Eq. (17) and fits for different $n$; left column $n = 1$, middle column $n = 3$ and right column $n = 5$: The first row shows the SD (blue solid line) together with a fit according to the parameters given in Table V of the SI (black, dashed). The insets show the difference between the original SD and the approximations. Second row: SD divided by $\omega^2$. Rows three to five: Corresponding BCFs for three temperatures using the Padé approximation of the hyperbolic cotangent. Blue and red correspond to the exact real and imaginary parts, respectively. The gray dashed/dotted curves are the approximations based on the Tables VI, VII, VIII of the SI. In the insets the differences are shown.

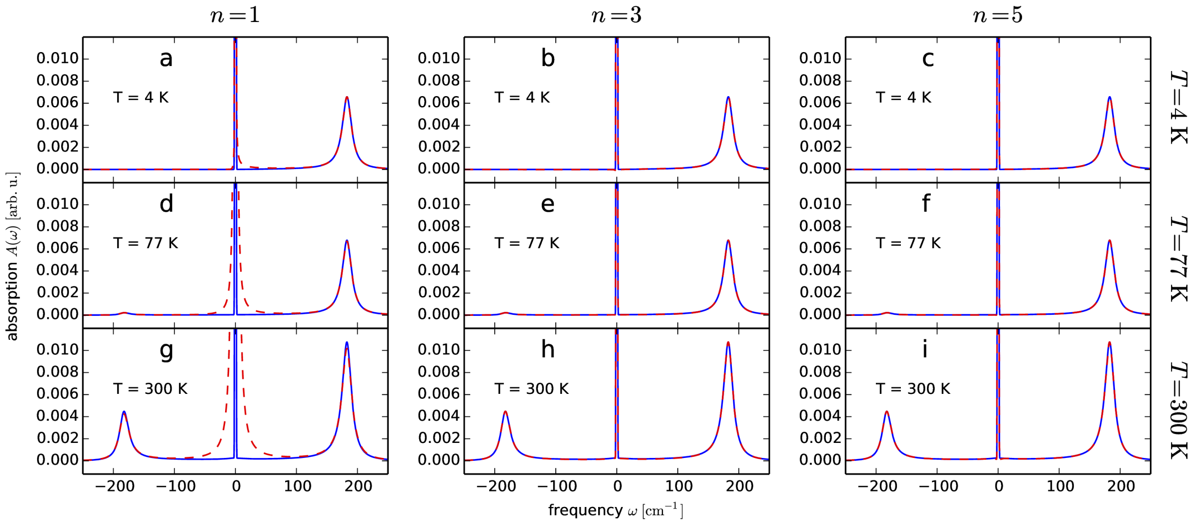


Figure 4 (SI): Absorption spectra for the SD of the damped vibrational mode according to Eq. (17), which is shown in Fig. 3 (a). The solid blue curve is the exact spectrum and the dashed red curve the one obtained from our fit. In the left column (panels (a), (d), (g)) the fit was performed with $n = 1$, in the middle column (panels (b), (e), (h)) with $n = 3$ and in the right column (panels (c), (f), (i)) with $n = 5$. The parameters for the respective fits are given in Tables VI, VII, VIII of the SI. The first row is for $T = 4$ K, the second for 77 K and the third for 300 K.

# 3 Combined SD (Background + Vibrational Mode)

Typically the SD of pigments in an (protein) environment consists of a broad background combined with peaks belonging to molecular vibrations. As a simple example we consider the sum $J(\omega) = J_{\mathrm{vib}}(\omega) + J_{\mathrm{bg}}(\omega)$, where $J_{\mathrm{vib}}(\omega)$ is the SD of the damped vibrational mode we considered in section 2 of this SI and $J_{\mathrm{bg}}(\omega)$ is the log-normal SD we considered in section 1 of this SI. We approximate the resulting spectral density by the sum of the fit functions used in section 1.1 and in section 2.1 of this SI.

## 3.1 Fits for the combined SD

In Table IX (SI) we provide the parameters for our fits to the combined SD, which is the sum of the log-normal background SD and the SD of the damped vibrational mode. For $n = 3$ and $n = 5$ we thus have 2 summands in Eq. (3). The parameters of both summands for the resulting fit we directly take from Tables I and V of this SI.

| | | $n = 1$ | $n = 3$ | $n = 5$ |
|---|---|---|---|---|
| $p_1$ | | 2.4339e+08 | 9.6501e+03 | 1.2700e+04 |
| | $\omega_{1_1}$ | 183.02+9.1263j | 183.05+9.1885j | 183.05+9.1738j |
| | $\omega_{1_2}$ | 261.23+139.66j | 95.468+161.08j | 67.569+178.12j |
| | $\omega_{1_3}$ | | | 1.7613+11.123j |
| | | | | |
| $p_2$ | | 3.6981e+09 | 1.7661e+10 | 2.4229e+05 |
| | $\omega_{2_1}$ | 125.69+65.995j | 14.709+29.995j | 5.5219+11.255j |
| | $\omega_{2_2}$ | 297.83+222.87j | 41.127+91.783j | 15.443+34.436j |
| | $\omega_{2_3}$ | | 137.60+272.05j | 51.693+102.07j |
| | | | | |
| $p_3$ | | 3.4283e+05 | | |
| | $\omega_{3_1}$ | 24.177+6.8901j | | |
| | $\omega_{3_2}$ | 61.146+7.7632j | | |
| | | | | |
| $p_4$ | | 5.9692e+05 | | |
| | $\omega_{4_1}$ | 33.176+10.937j | | |
| | $\omega_{4_2}$ | 52.446+11.077j | | |
| | | | | |
| $p_5$ | | 3.2796e+07 | | |
| | $\omega_{5_1}$ | 112.26+36.733j | | |
| | $\omega_{5_2}$ | 65.201+22.859j | | |
| | | | | |

Table IX (SI): Fit parameters for the combined SD according to Eqs. (3), (4) for three different scaling parameters $n \in \{1, 3, 5\}$. The values are directly taken from Tables I and V of this SI.

## 3.2 Resulting parameters for the BCFs corresponding to our fits of the combined SD

Here, we provide the coefficients of the exponential decomposition Eq. (2) of the BCF for the different fits of the combined SD from Table IX (SI) for different temperatures $T \in \{4\ \text{K}, 77\ \text{K}, 300\ \text{K}\}$.

### 3.2.1 Parameters for the BCF corresponding to the fit for n=1

In Table X (SI) we list the parameters of the exponential decomposition Eq. (2) of the BCF (according to Eq. (6)) for the scaling parameter $n = 1$, i.e. an ohmic fit function with a linear behavior at frequency zero. For $T = 4$ K we take 9 Padé expansion terms for the hyperbolic cotangent into account, for $T = 77$ K we take 2 terms and for $T = 300$ K we take 1 term.

### 3.2.2 Parameters for the BCF corresponding to the fit for n=3

In Table XI (SI) we list the parameters of the exponential decomposition Eq. (2) of the BCF (according to Eq. (6)) for the scaling parameter $n = 3$, i.e. a superohmic fit function with a cubic behavior at frequency zero. For $T = 4$ K we take 14 Padé expansion terms for the hyperbolic cotangent into account, for $T = 77$ K we take 2 terms and for $T = 300$ K we take 1 term.

### 3.2.3 Parameters for the BCF corresponding to the fit for n=5

In Table XII (SI) we list the parameters of the exponential decomposition Eq. (2) of the BCF (according to Eq. (6)) for the scaling parameter $n = 5$, i.e. a superohmic fit function with a behavior proportional to $\omega^5$ at frequency zero. For $T = 4$ K we take 13 Padé expansion terms for the hyperbolic cotangent into account, for $T = 77$ K we take 3 terms and for $T = 300$ K we take 1 term.

| $T = 4$ K | $p_m$ | $\omega_m$ |
|---|---|---|
| | -2.1023e-28+3.7609e-27j | 1.8302e+02+9.1263e+00j |
| | 2.9190e-41-1.7778e-41j | 2.6123e+02+1.3966e+02j |
| | -4.7371e-18+1.5626e-17j | 1.2569e+02+6.5995e+01j |
| | 6.1816e-45-1.2636e-45j | 2.9783e+02+2.2287e+02j |
| | -2.9753e-03-4.8109e-03j | 2.4177e+01+6.8901e+00j |
| | -8.4164e-09+4.3624e-10j | 6.1146e+01+7.7632e+00j |
| | -6.3505e-04-3.3146e-05j | 3.3176e+01+1.0937e+01j |
| | 8.0172e-08+6.0801e-07j | 5.2446e+01+1.1077e+01j |
| | -3.8931e-16-1.5628e-16j | 1.1226e+02+3.6733e+01j |
| | 6.1569e-09-2.4373e-08j | 6.5201e+01+2.2859e+01j |
| | 1.0411e+03-5.8197e+01j | -1.8302e+02+9.1263e+00j |
| | -3.5444e+01+5.8197e+01j | -2.6123e+02+1.3966e+02j |
| | 6.8473e+02-2.0758e+02j | -1.2569e+02+6.5995e+01j |
| | -4.2431e+01+2.0758e+02j | -2.9783e+02+2.2287e+02j |
| | 3.1737e+01-1.1716e+01j | -2.4177e+01+6.8901e+00j |
| | 2.7648e+01+1.1721e+01j | -6.1146e+01+7.7632e+00j |
| | 6.4290e+01-7.2376e+01j | -3.3176e+01+1.0937e+01j |
| | 6.2428e+01+7.2376e+01j | -5.2446e+01+1.1077e+01j |
| | 8.9275e+01+2.2240e+02j | -1.1226e+02+3.6733e+01j |
| | 3.1439e+02-2.2240e+02j | -6.5201e+01+2.2859e+01j |
| | -1.0412e+01-3.7039e-15j | 0.0000e+00+1.7468e+01j |
| | -1.2904e+01+1.2346e-15j | 0.0000e+00+3.4936e+01j |
| | -1.3537e+01+1.2346e-15j | 0.0000e+00+5.2404e+01j |
| | -1.3174e+01+6.1737e-16j | 0.0000e+00+6.9873e+01j |
| | -1.2390e+01+9.4550e-16j | 0.0000e+00+8.7421e+01j |
| | -1.4318e+01+1.7123e-15j | 0.0000e+00+1.0743e+02j |
| | -1.8563e+01+0.0000e+00j | 0.0000e+00+1.4226e+02j |
| | -1.0449e+00+2.5858e-15j | 0.0000e+00+2.2861e+02j |
| | 1.3576e+01-7.4115e-16j | 0.0000e+00+6.7400e+02j |
| $T = 77$ K | $p_m$ | $\omega_m$ |
| | 3.4997e+01-4.2350e+00j | 1.8302e+02+9.1263e+00j |
| | 9.6513e-03+5.1361e-01j | 2.6123e+02+1.3966e+02j |
| | 3.6076e+01-6.0291e+01j | 1.2569e+02+6.5995e+01j |
| | 7.6069e-01+2.7730e-01j | 2.9783e+02+2.2287e+02j |
| | 5.7018e+01+3.9485e-01j | 2.4177e+01+6.8901e+00j |
| | 1.1421e+01-8.0391e+00j | 6.1146e+01+7.7632e+00j |
| | 9.8212e+01+4.3080e+01j | 3.3176e+01+1.0937e+01j |
| | 2.1056e+01-5.2196e+01j | 5.2446e+01+1.1077e+01j |
| | -1.2323e+01-2.9946e+01j | 1.1226e+02+3.6733e+01j |
| | 1.5365e+02+3.4506e+00j | 6.5201e+01+2.2859e+01j |
| | 1.0761e+03-5.3962e+01j | -1.8302e+02+9.1263e+00j |
| | -3.5434e+01+5.7683e+01j | -2.6123e+02+1.3966e+02j |
| | 7.2081e+02-1.4729e+02j | -1.2569e+02+6.5995e+01j |
| | -4.1670e+01+2.0730e+02j | -2.9783e+02+2.2287e+02j |
| | 8.8758e+01-1.2116e+01j | -2.4177e+01+6.8901e+00j |
| | 3.9069e+01+1.9760e+01j | -6.1146e+01+7.7632e+00j |
| | 1.6250e+02-1.1546e+02j | -3.3176e+01+1.0937e+01j |
| | 8.3484e+01+1.2457e+02j | -5.2446e+01+1.1077e+01j |
| | 7.6952e+01+2.5234e+02j | -1.1226e+02+3.6733e+01j |
| | 4.6804e+02-2.2585e+02j | -6.5201e+01+2.2859e+01j |
| | 2.2699e+01+0.0000e+00j | 0.0000e+00+3.3748e+02j |
| | 2.9558e+00+0.0000e+00j | 0.0000e+00+1.0436e+03j |
| $T = 300$ K | $p_m$ | $\omega_m$ |
| | 7.4090e+02-1.4099e+01j | 1.8302e+02+9.1263e+00j |
| | -2.4251e+01-3.1531e+00j | 2.6123e+02+1.3966e+02j |
| | 7.1876e+02-2.7319e+02j | 1.2569e+02+6.5995e+01j |
| | -5.5725e+01-3.7440e+00j | 2.9783e+02+2.2287e+02j |
| | 2.6423e+02+1.5684e+01j | 2.4177e+01+6.8901e+00j |
| | 7.4677e+01-4.5456e+01j | 6.1146e+01+7.7632e+00j |
| | 4.6811e+02+2.5520e+02j | 3.3176e+01+1.0937e+01j |
| | 1.4983e+02-2.9070e+02j | 5.2446e+01+1.1077e+01j |
| | -9.7366e+00-3.1959e+02j | 1.1226e+02+3.6733e+01j |
| | 9.6639e+02+2.1691e+02j | 6.5201e+01+2.2859e+01j |

| | | |
|---|---|---|
| | 1.7820e+03-4.4097e+01j<br>-5.9695e+01+6.1350e+01j<br>1.4035e+03+6.5615e+01j<br>-9.8156e+01+2.1132e+02j<br>2.9597e+02-2.7405e+01j<br>1.0232e+02+5.7177e+01j<br>5.3240e+02-3.2757e+02j<br>2.1226e+02+3.6307e+02j<br>7.9539e+01+5.4199e+02j<br>1.2808e+03-4.3931e+02j<br>5.9823e-01+0.0000e+00j | -1.8302e+02+9.1263e+00j<br>-2.6123e+02+1.3966e+02j<br>-1.2569e+02+6.5995e+01j<br>-2.9783e+02+2.2287e+02j<br>-2.4177e+01+6.8901e+00j<br>-6.1146e+01+7.7632e+00j<br>-3.3176e+01+1.0937e+01j<br>-5.2446e+01+1.1077e+01j<br>-1.1226e+02+3.6733e+01j<br>-6.5201e+01+2.2859e+01j<br>0.0000e+00+1.6151e+03j |

Table X (SI): Parameters for the BCF decomposition Eq. (2) for our fit of the combined SD with $n = 1$ for 3 different temperatures $T \in \{4\ \mathrm{K}, 77\ \mathrm{K}, 300\ \mathrm{K}\}$.

| $T = 4$ K | $p_m$ | $\omega_m$ |
|---|---|---|
| | -2.2775e-28+4.3464e-27j | 1.8305e+02+9.1885e+00j |
| | -7.5986e-14+1.7536e-14j | 9.5468e+01+1.6108e+02j |
| | -1.8461e+00-4.0609e+00j | 1.4709e+01+2.9995e+01j |
| | -2.2573e-05-1.1358e-03j | 4.1127e+01+9.1783e+01j |
| | 7.9254e-20-9.9991e-20j | 1.3760e+02+2.7205e+02j |
| | 1.0494e+03-5.4989e+01j | -1.8305e+02+9.1885e+00j |
| | -2.9849e+01+5.4989e+01j | -9.5468e+01+1.6108e+02j |
| | -7.1391e+02-5.2398e+02j | -1.4709e+01+2.9995e+01j |
| | 3.0202e+03-2.2080e+01j | -4.1127e+01+9.1783e+01j |
| | -6.9406e+02+5.5012e+02j | -1.3760e+02+2.7205e+02j |
| | 4.6863e+01+8.8296e-15j | 0.0000e+00+1.7468e+01j |
| | 2.3386e+02-2.3546e-14j | 0.0000e+00+3.4936e+01j |
| | 2.1653e+01+0.0000e+00j | 0.0000e+00+5.2404e+01j |
| | -1.6566e+02-2.3546e-14j | 0.0000e+00+6.9873e+01j |
| | -2.8744e+02+0.0000e+00j | 0.0000e+00+8.7341e+01j |
| | -2.7376e+02+0.0000e+00j | 0.0000e+00+1.0481e+02j |
| | -1.7777e+02+2.7048e-14j | 0.0000e+00+1.2228e+02j |
| | -9.6711e+01-1.2008e-14j | 0.0000e+00+1.3983e+02j |
| | -4.9187e+01+0.0000e+00j | 0.0000e+00+1.5899e+02j |
| | -2.5440e-01+0.0000e+00j | 0.0000e+00+1.8591e+02j |
| | 8.3598e+01+1.3619e-14j | 0.0000e+00+2.3089e+02j |
| | 1.5392e+02-3.2185e-15j | 0.0000e+00+3.1547e+02j |
| | 4.4467e+01+6.1264e-15j | 0.0000e+00+5.1766e+02j |
| | -1.1993e+00-4.8109e-16j | 0.0000e+00+1.5413e+03j |
| $T = 77$ K | $p_m$ | $\omega_m$ |
| | 3.5231e+01-4.4310e+00j | 1.8305e+02+9.1885e+00j |
| | 3.3791e+00+8.3508e+00j | 9.5468e+01+1.6108e+02j |
| | 5.7203e+02+1.1116e+03j | 1.4709e+01+2.9995e+01j |
| | -6.2342e+02-1.0325e+03j | 4.1127e+01+9.1783e+01j |
| | 2.5263e+01-6.4693e+01j | 1.3760e+02+2.7205e+02j |
| | 1.0846e+03-5.0558e+01j | -1.8305e+02+9.1885e+00j |
| | -2.6470e+01+4.6638e+01j | -9.5468e+01+1.6108e+02j |
| | -1.4004e+02-1.6396e+03j | -1.4709e+01+2.9995e+01j |
| | 2.3968e+03+1.0105e+03j | -4.1127e+01+9.1783e+01j |
| | -6.6879e+02+6.1481e+02j | -1.3760e+02+2.7205e+02j |
| | 3.6486e+02+3.1994e-14j | 0.0000e+00+3.3748e+02j |
| | 1.9409e+00+3.4522e-15j | 0.0000e+00+1.0436e+03j |
| $T = 300$ K | $p_m$ | $\omega_m$ |
| | 7.4643e+02-1.7186e+01j | 1.8305e+02+9.1885e+00j |
| | -5.2331e+01+2.0795e+01j | 9.5468e+01+1.6108e+02j |
| | 1.3477e+03+5.1719e+03j | 1.4709e+01+2.9995e+01j |
| | 1.1413e+03-5.5949e+03j | 4.1127e+01+9.1783e+01j |
| | -1.8408e+02+4.2029e+02j | 1.3760e+02+2.7205e+02j |
| | 1.7958e+03-3.7802e+01j | -1.8305e+02+9.1885e+00j |
| | -8.2180e+01+3.4194e+01j | -9.5468e+01+1.6108e+02j |
| | 6.3567e+02-5.7000e+03j | -1.4709e+01+2.9995e+01j |
| | 4.1615e+03+5.5728e+03j | -4.1127e+01+9.1783e+01j |
| | -8.7814e+02+1.2983e+02j | -1.3760e+02+2.7205e+02j |
| | -1.2523e+00-1.6872e-15j | 0.0000e+00+1.6151e+03j |

Table XI (SI): Parameters for the BCF decomposition Eq. (2) for our fit of the combined SD with $n = 3$ for 3 different temperatures $T \in \{4\text{ K}, 77\text{ K}, 300\text{ K}\}$.

| $T = 4$ K | $p_m$ | $\omega_m$ |
|---|---|---|
| | -2.2071e-28+4.2011e-27j | 1.8305e+02+9.1738e+00j |
| | -1.6149e-09-1.9259e-11j | 6.7569e+01+1.7812e+02j |
| | -2.9801e-03+5.0132e-03j | 1.7613e+00+1.1123e+01j |
| | 3.2261e+00+3.2153e+00j | 5.5219e+00+1.1255e+01j |
| | -3.4409e+00+2.6437e+00j | 1.5443e+01+3.4436e+01j |
| | 1.9050e-05+1.6683e-05j | 5.1693e+01+1.0207e+02j |
| | 1.0475e+03-5.5031e+01j | -1.8305e+02+9.1738e+00j |
| | -1.8328e+01+5.5024e+01j | -6.7569e+01+1.7812e+02j |
| | 1.0821e-02+1.9142e-03j | -1.7613e+00+1.1123e+01j |
| | 3.9637e+00+3.2956e+01j | -5.5219e+00+1.1255e+01j |
| | -7.5276e+02-8.3121e+02j | -1.5443e+01+3.4436e+01j |
| | 2.9044e+03+7.9239e+02j | -5.1693e+01+1.0207e+02j |
| | -2.0663e+01+7.0162e-15j | 0.0000e+00+1.7468e+01j |
| | 2.5308e+02+7.0162e-15j | 0.0000e+00+3.4936e+01j |
| | 1.8345e+02+5.3279e-14j | 0.0000e+00+5.2404e+01j |
| | -1.0139e-01+0.0000e+00j | 0.0000e+00+6.9873e+01j |
| | -1.3595e+02+6.8518e-14j | 0.0000e+00+8.7341e+01j |
| | -2.1613e+02-1.7760e-14j | 0.0000e+00+1.0481e+02j |
| | -2.1992e+02+8.2637e-15j | 0.0000e+00+1.2229e+02j |
| | -1.9447e+02+1.9868e-14j | 0.0000e+00+1.4041e+02j |
| | -1.9204e+02+0.0000e+00j | 0.0000e+00+1.6370e+02j |
| | -1.7694e+02+1.1191e-14j | 0.0000e+00+2.0218e+02j |
| | -1.3942e+02+1.9572e-14j | 0.0000e+00+2.7515e+02j |
| | -8.7000e+01+2.4917e-14j | 0.0000e+00+4.5041e+02j |
| | -2.9521e+01+0.0000e+00j | 0.0000e+00+1.3395e+03j |
| $T = 77$ K | $p_m$ | $\omega_m$ |
| | 3.5171e+01-4.4084e+00j | 1.8305e+02+9.1738e+00j |
| | 5.7771e+00+1.1454e+01j | 6.7569e+01+1.7812e+02j |
| | -2.9000e-02-6.6243e-02j | 1.7613e+00+1.1123e+01j |
| | -1.3697e+02-5.3053e+01j | 5.5219e+00+1.1255e+01j |
| | 9.4904e+02+1.0160e+03j | 1.5443e+01+3.4436e+01j |
| | -7.6670e+02-5.9391e+02j | 5.1693e+01+1.0207e+02j |
| | 1.0827e+03-5.0622e+01j | -1.8305e+02+9.1738e+00j |
| | -1.2550e+01+4.3570e+01j | -6.7569e+01+1.7812e+02j |
| | -1.5199e-02+7.3170e-02j | -1.7613e+00+1.1123e+01j |
| | -1.3623e+02+8.9224e+01j | -5.5219e+00+1.1255e+01j |
| | 1.9972e+02-1.8446e+03j | -1.5443e+01+3.4436e+01j |
| | 2.1377e+03+1.3863e+03j | -5.1693e+01+1.0207e+02j |
| | -2.4323e+02+0.0000e+00j | 0.0000e+00+3.3627e+02j |
| | -3.4999e+01-1.3008e-14j | 0.0000e+00+6.9350e+02j |
| | -1.3825e+01+2.6404e-14j | 0.0000e+00+1.9330e+03j |
| $T = 300$ K | $p_m$ | $\omega_m$ |
| | 7.4510e+02-1.6966e+01j | 1.8305e+02+9.1738e+00j |
| | -5.0828e+01+2.2055e+01j | 6.7569e+01+1.7812e+02j |
| | -9.3577e-02-2.6892e-01j | 1.7613e+00+1.1123e+01j |
| | -5.3491e+02-2.5799e+02j | 5.5219e+00+1.1255e+01j |
| | 2.8416e+03+5.2311e+03j | 1.5443e+01+3.4436e+01j |
| | -2.5598e+02-4.8763e+03j | 5.1693e+01+1.0207e+02j |
| | 1.7926e+03-3.8065e+01j | -1.8305e+02+9.1738e+00j |
| | -6.9156e+01+3.2969e+01j | -6.7569e+01+1.7812e+02j |
| | -7.9776e-02+2.7585e-01j | -1.7613e+00+1.1123e+01j |
| | -5.3417e+02+2.9416e+02j | -5.5219e+00+1.1255e+01j |
| | 2.0923e+03-6.0596e+03j | -1.5443e+01+3.4436e+01j |
| | 2.6484e+03+5.6687e+03j | -5.1693e+01+1.0207e+02j |
| | -2.0621e+01-2.2386e-14j | 0.0000e+00+1.6151e+03j |

Table XII (SI): Parameters for the BCF decomposition Eq. (2) for our fit of the combined SD with $n = 5$ for 3 different temperatures $T \in \{4\ \mathrm{K}, 77\ \mathrm{K}, 300\ \mathrm{K}\}$.

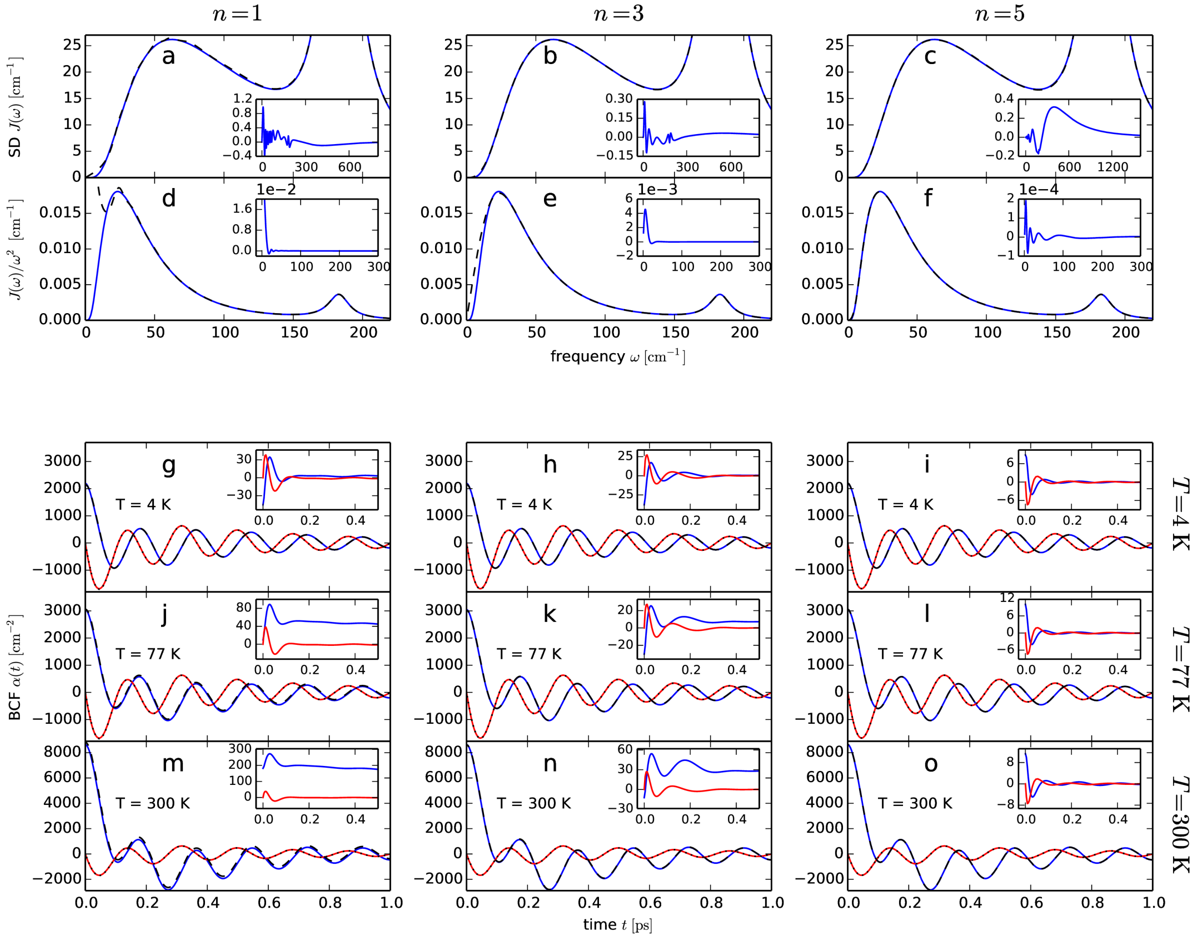


Figure 5 (SI): Combined SD and fits for different $n$; left column $n = 1$, middle column $n = 3$ and right column $n = 5$: The first row shows the SD (blue solid line) together with a fit according to the parameters given in Table IX of the SI (black, dashed). The insets show the difference between the original SD and the approximations. Second row: SD divided by $\omega^2$. Rows three to five: Corresponding BCFs for three temperatures using the Padé approximation of the hyperbolic cotangent. Blue and red correspond to the exact real and imaginary parts, respectively. The gray dashed/dotted curves are the approximations based on the Tables X, XI, XII of the SI. In the insets the differences are shown.

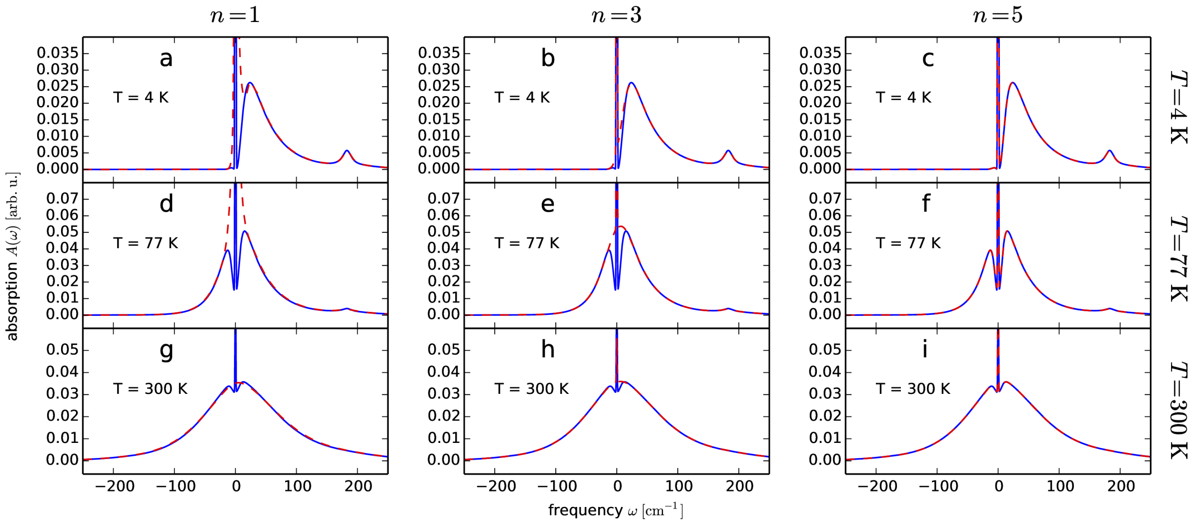


Figure 6 (SI): Absorption spectra for the combined SD, which is shown in Fig. 5 of the SI. The solid blue curve is the exact spectrum and the dashed red curve the one obtained from our fit. In the left column (panels (a), (d), (g)) the fit was performed with $n = 1$, in the middle column (panels (b), (e), (h)) with $n = 3$ and in the right column (panels (c), (f), (i)) with $n = 5$. The parameters for the respective fits are given in Tables X, XI, XII of the SI. The first row is for $T = 4$ K, the second for 77 K and the third for 300 K.
